# Supplementary material for: Universality for the directed configuration model: metric space convergence of the strongly connected components at criticality
Source: arXiv:2105.11434 source file (2021-11-02)
Supplement: Supplementary file 2 [file Backup_Appendix_measure_change.tex]

\section{Analysis of the measure change}
\label{sec:measure-change-2}

We recall some notation and the lemma we wish to prove. Recall that $\vD_1, \vD_2, \ldots$ are i.i.d.\ copies of $(D^-, D^+)$ a $\N \times \N$-valued random variable. We assume $\E[D^-] = \E[D^+]$ and call this quantity $\mu$. We will use the notation
\begin{equation*}
    \Xi^{\pm}_n = \textstyle \sum_{i=1}^n D^{\pm}_i
    \quad \text{and} \quad
    \Delta_n = \Xi^-_n - \Xi^+_n.
\end{equation*}
We defined
\begin{equation*}
    \cI_n = \{ i \in [n] : D_i^- > 0 \} \quad \text{and} \quad R_n = \abs{\cI_n}.
\end{equation*}
Then $\hat{\vD}_{n, 1}, \ldots, \hat{\vD}_{n, R_n}$ are the elements of $\{\vD_i : u \in \cI_n\}$ in order of discovery according to the eDFS procedure. We will compare this against a sequence of i.i.d.\ $\N \times \N$-valued random variables $\vZ_1, \vZ_2, \ldots$, where for each $i \geq 1$ $\vZ_i$ has law
\begin{equation*}
    \P(Z_i^- = k^-, Z_i^+ = k^+) = \frac{k^-}{\mu} \P(D^- = k^-, D^+ = k^+).
\end{equation*}
Let $\lambda_{\pm} = \E[Z^{\pm}_1]$. We have $\nu_- = \lambda_- - 1$ and under the criticality condition we have $\lambda_+ = 1$. We used the notation
\begin{equation*}
    Y^{\pm}(n) = \sum_{i=1}^n (Z^{\pm}_i - 1).
\end{equation*}
The following theorem asserts the existence of a measure change under conditioning of equal in- and out-degrees and, moreover, it gives the scaling limit of the Radon--Nikodym derivative.

\measurechange*

We observe that the criticality condition $\lambda_+ = 1$ is, in fact, not necssary for this to hold, and instead prove the following more general result.

\begin{lemma}
    \label{prop:measure-change-no-crit}
    Define the centered random walks
    \begin{equation*}
        V^{\pm}(n) = \sum_{i=1}^n (Z^{\pm} - \lambda_{\pm}).
    \end{equation*}
    Then using the notation of \cref{thm:measure-change},
    \begin{align*}
        &\left( 
            \Phi(n, \floor{T n^{2/3}}),
            \left(
                n^{-1/3} V^-\left( \floor{n^{2/3} t} \right),
                n^{-1/3} V^+\left( \floor{n^{2/3} t} \right)
            \right)_{t \in [0, T]}
        \right) \\
        & \hspace{23em} \todist \left( 
            \Phi(T),
            (\sigma_- W^-_t, \sigma_+ W^+_t)_{t \in [0, T]}
        \right)
    \end{align*}
    as $n \to \infty$, even in absence of the criticality condition.
\end{lemma}

\cref{thm:measure-change} then follows as a direct corollary of \cref{prop:measure-change-no-crit} by noting that
\begin{equation*}
    \left( 
        Y^-(n), Y^+(n)
     \right) =
    \left( 
        V^-(n) + n \nu_-, V^+(n)
     \right)
\end{equation*}
and using the continuous mapping theorem. The proof of this result is based upon the proof of \cite[Lemma~6.7]{conchon--kerjanStableGraphMetric2021}, but considerably more work is required in order to deal with the asymptotically singular conditioning.

\subsection{Exact form of the measure change}

We first examine the exact law of the reordering of the vertices. Let $\Sigma_n: [R_n] \to \cI_n$ be the random bijection such that $\hat{\vD}_{n, i} = \vD_{\Sigma_n(i)}$ for $i = 1, \ldots, R_n$.

\begin{lemma}
    $\Sigma_n$ has law
    \begin{equation*}
        \P(\Sigma_n = \sigma \mid \vD_1, \ldots, \vD_n)
        = \prod_{i=1}^{R_n} \frac{D^-_{\sigma(i)}}{\sum_{j=i}^{R_n} D^-_{\sigma(j)}}.
    \end{equation*}
\end{lemma}
\begin{proof}
    The key idea is that the eDFS procedure can be adapted to carry out the pairing of in- and out-half-edges that is used the define the configuration model. Instead of keeping a stack of edges, we keep a stack of out-half-edges. When we examine an out-half-edge, we sample the head of the half-edge by picking a uniform choice from the unpaired in-half-edges. Thus when we are exploring a new vertex we are picking it with probability proportional to its in-degree. This is also why we start new out-components by picking a vertex with probability proportional to its in-degree.

    Hence the probability of exploring the vertex $v_{\sigma(1)}$ is
    \begin{equation*}
        \frac{D_{\sigma(1)}^{-}}{\sum_{j=1}^{R_n} D_{\sigma(j)}}.
    \end{equation*}
    Conditional on the $\Sigma_n(1) = \sigma(1)$, the probability the next vertex we explore is $v_{\sigma(2)}$ is
    \begin{equation*}
        \frac{D_{\sigma(2)}^{-}}{\sum_{j=2}^{R_n} D_{\sigma(j)}}.
    \end{equation*}
    Continuing inductively gives the desired result.
\end{proof}

Next we establish the form of the measure change when we condition on the exact value of $R_n$ but not $\Delta_n = 0$.

\begin{lemma}
    \label{lem:exact-measure-change-no-conditioning}
    For all integers $0 \leq r \leq n$ and test functions $u: (\N \times \N)^r \times \N \to \R$,
    \begin{equation*}
        \E \left[ u\left( 
            \hat{\vD}_{n, 1}, \ldots, \hat{\vD}_{n, r}, \textstyle \sum_{i \in \cI_n^c} D_i^+
        \right) \,\middle\vert\, R_n = r \right] \\
        =
        \E \left[
            u\left( \vZ_1, \ldots, \vZ_r, \textstyle \sum_{i = 1}^{n-r} E_i^+ \right)
            \psi_r(\vZ_1, \ldots, \vZ_r)
        \right]
    \end{equation*}
    where
    \begin{equation*}
        \psi_r(\vk_1, \ldots, \vk_r) =
        \frac{1}{p^r} \prod_{i=1}^r \frac{(r - i + 1)\mu}{\sum_{j=i}^r k_i^-}.
    \end{equation*}
    and $E_1^+, E_2^+, \ldots$ are of i.i.d.\ random variables such that $E_i^+$ has the same distribution as $D^+$ conditioned on $D^- = 0$ and $p = \P(\D^- > 0)$. We take the sequences $(E_i^+)_{i \geq 1}$ and $(\vZ_i)_{i \geq 1}$ to be independent.
\end{lemma}

\begin{proof}
    For any $\vk_1, \ldots, \vk_m \in \N^+ \times \N$ for all $i$ and $s \in \N$.
    \begin{align*}
        & \P\left(\hat{\vD}_{n, 1} = \vk_1, \ldots, \hat{\vD}_{n, r} = \vk_r, \textstyle \sum_{i \in \cI_n^c} D_i^+ = s, R_n = r \right) \\
        =& \sum_{\substack{I \subset [n] \\ \abs{I} = r}} \sum_{\sigma: [r] \to I}
        \P\left(\vD_{\Sigma_n(1)} = \vk_1, \ldots, \vD_{\Sigma_n(r)} = \vk_r, \textstyle \sum_{i \in \cI_n^c} D_i^+ = s, \cI_n = I, \Sigma_n = \sigma \right)
    \end{align*}
    where the second summation is taken over all bijections $\sigma: [r] \to I$. We examine a single summand.
    \begin{align*}
        &\P\left(\vD_{\Sigma_n(1)} = \vk_1, \ldots, \vD_{\Sigma_n(r)} = \vk_r, \textstyle \sum_{i \in \cI_n^c} D_i^+ = s, \cI_n = I, \Sigma_n = \sigma \right) \\
        =&\P\left(
            \vD_{\sigma(j)} = \vk_j\ \text{for $j = 1, \ldots, r$},
            \textstyle \sum_{i \in I^c} D_i^+ = s,
            D^-_i = 0\ \text{for $i \in I^c$},
            \Sigma_n = \sigma
            \right)  \\
        =& \prod_{i=1}^r \frac{k_i^-}{\sum_{j=i}^r k_j^-}
        \times \prod_{i=1}^r \lambda_{\vk_i}
        \times \P\left( 
            \textstyle \sum_{i \in I^c} D_i^+ = s,
            D^-_i = 0\ \text{for $i \in I^c$}
         \right).
    \end{align*}
    where $\lambda_{\vk} = \P(\vD_1 = \vk)$. We have
    \begin{equation*}
        \P\left( 
            \textstyle \sum_{i \in I^c} D_i^+ = s,
            D^-_i = 0\ \text{for $i \in I^c$}
         \right)
         = (1-p)^{n-r} \P\left( 
             \textstyle \sum_{i=1}^{n-r} E^+_i = s
          \right).
    \end{equation*}
    Also
    \begin{align*}
        \prod_{i=1}^r \frac{k_i^-}{\sum_{j=i}^r k_j^-} \times \prod_{i=1}^r \lambda_{\vk_i}
        &= \prod_{i=1}^r \frac{k_i^-}{\mu} \lambda_{\vk_i} \times \prod_{i=1}^r \frac{\mu}{\sum_{j=i}^r k_j^-} \\
        &= \P(\vZ_1 = \vk_1, \ldots, \vZ_r = \vk_r)
        \times \prod_{i=1}^r \frac{\mu}{\sum_{j=i}^r k_j^-}.
    \end{align*}
    Therefore
    \begin{align*}
        & \P\left(\hat{\vD}_{n, 1} = \vk_1, \ldots, \hat{\vD}_{n, r} = \vk_r, \textstyle \sum_{i \in \cI_n^c} D_i^+ = s, R_n = r \right) \\
        =& \binom{n}{r} \times r!
        \times \prod_{i=1}^r \frac{\mu}{\sum_{j=i}^r k_j^-} \times (1-p)^{n-r}
        \times \P\left(\vZ_1 = \vk_1, \ldots, \vZ_r = \vk_r, \textstyle \sum_{i=1}^{n-r} E_i^+ = s \right) \\
        =& \binom{n}{r} p^r (1-p)^{n-r} \times \frac{1}{p^r} \prod_{i=1}^r \frac{(r-i+1) \mu}{\sum_{j=i}^r k_i^-}
        \times \P\left(\vZ_1 = \vk_1, \ldots, \vZ_r = \vk_r, \textstyle \sum_{i=1}^{n-r} E_i^+ = s \right).
    \end{align*}
    Finally dividing by $\P(R_n = r) = \binom{n}{r} p^r (1-p)^{n-r}$ gives the desired measure change.
\end{proof}

Using the previous lemma we can prove existence and give the exact form of the desired measure change $\phi^n_m$.

\begin{lemma}
    \label{lem:exact-measure-change}
    For all $m \leq n$ and test functions $u: (\N \times \N)^m \to \R$,
    \begin{equation*}
        \E \left[
            u\left( \hat{\vD}_{n, 1}, \ldots, \hat{\vD}_{n, m} \right)
            \,\middle\vert\,
            R_n \geq m,
            \Delta_n = 0
        \right] \\
        =
        \E \left[
            u\left( \vZ_1, \ldots, \vZ_m \right)
            \phi^n_m(\vZ_1, \ldots, \vZ_m)
        \right],
    \end{equation*}
    where
    \begin{align*}
        \phi^n_m(\vk_1, \ldots, \vk_m) =
        \frac{1}{\P(R_n \geq m, \Delta_n = 0)} \E\left[ 
            \one \left\{ \Delta_{n-m} = \sum_{i=1}^m (k_i^+ - k_i^-) \right\}
            \prod_{i=1}^m \frac{(n - i + 1) \mu}{\sum_{j=1}^m k_j^- + \Xi_{n-m}^-}
        \right].
    \end{align*}
\end{lemma}

\begin{proof}
    By \cref{lem:exact-measure-change-no-conditioning}, for all $r \geq m$
    \begin{align*}
        &\E \left[ 
            u\left( 
                \hat{\vD}_{n, 1}, \ldots, \hat{\vD}_{n, m}
             \right)
            \one\{\Delta_n = 0\}
            \, \middle\vert \,
            R_n = r
         \right] \\
        =&\E \left[ 
            u\left( \vZ_1, \ldots, \vZ_m \right)
            \one \left\{ 
                \sum_{i=1}^r (Z_i^- - Z_i^+) - \sum_{i=1}^{n-r} E_i^+ = 0
             \right\}
             \frac{1}{p^r} \prod_{i=1}^r \frac{(r - i + 1) \mu}{\sum_{j=i}^r Z_j^-}
         \right] \\
        =&\E \left[ 
            u\left( \vZ_1, \ldots, \vZ_m \right)
            \E \left[ 
                \one \left\{ 
                    \sum_{i=1}^r (Z_i^- - Z_i^+) - \sum_{i=1}^{n-r} E_i^+ = 0
                \right\}
                \frac{1}{p^r} \prod_{i=1}^r \frac{(r - i + 1) \mu}{\sum_{j=i}^r Z_j^-}
                \, \middle \lvert \,
                \vZ_1, \ldots, \vZ_m
             \right]
         \right] \\
        =&\E \left[ 
            u\left( \vZ_1, \ldots, \vZ_m \right)
            \tilde{\gamma}^{n, m}_r (\vZ_1, \ldots, \vZ_m)
         \right],
    \end{align*}
    where
    \begin{align*}
        \tilde{\gamma}^{n, m}_r (\vk_1, \ldots, \vk_m)
        &= \E \Bigg[ 
            \one \left\{ 
                \sum_{i=m+1}^r (Z_i^- - Z_i^+) - \sum_{i=1}^{n-r} E_i^+ = \sum_{i=1}^m (k_i^+ - k_i^-)
            \right\} \times \\
            &\hspace{5em}
            \frac{1}{p^m} \prod_{i=1}^m \frac{(r - i + 1) \mu}{\sum_{j=i}^m k_j^- + \sum_{j=m+1}^r Z_j^-}
            \frac{1}{p^{m-r}} \prod_{i=m+1}^r \frac{(r - i + 1) \mu}{\sum_{j=i}^r Z_j^-}
        \Bigg] \\
        &= \E \Bigg[ 
            \one \left\{ 
                \sum_{i=1}^{r-m} (Z_i^- - Z_i^+) - \sum_{i=1}^{n-r} E_i^+ = \sum_{i=1}^m (k_i^+ - k_i^-)
            \right\} \times \\
            &\hspace{5em}
            \frac{1}{p^m} \prod_{i=1}^m \frac{(r - i + 1) \mu}{\sum_{j=i}^m k_j^- + \sum_{j=1}^{r-m} Z_j^-}
            \frac{1}{p^{m-r}} \prod_{i=1}^{r-m} \frac{(r - m - i + 1) \mu}{\sum_{j=i}^{r-m} Z_j^-}
        \Bigg],
    \end{align*}
    since $(\vZ_i)_{i=m+1}^r$ has the same law as $(\vZ_i)_{i=1}^{r-m}$. Then applying \cref{lem:exact-measure-change-no-conditioning} again shows that
    \begin{align*}
        \tilde{\gamma}^{n, m}_r (\vk_1, \ldots, \vk_m)
        &= \E \Bigg[ 
            \one \left\{ 
                \sum_{i=1}^{r-m} (\hat{D}_{n-m,i}^- - \hat{D}_{n-m,i}^+) - \sum_{i \in \cI_{n-m}^c} D_i^+ = \sum_{i=1}^m (k_i^+ - k_i^-)
            \right\} \times \\
            &\hspace{8em}
            \frac{1}{p^m} \prod_{i=1}^m \frac{(r - i + 1) \mu}{\sum_{j=i}^m k_j^- + \sum_{j=1}^{r-m} \hat{D}_{n-m,j}^-}
            \Biggm|
            R_{n-m} = r-m
        \Bigg].
    \end{align*}
    Conditional on $R_{n-m} = r-m$, we have
    \begin{equation*}
        \sum_{j=1}^{r-m} (\hat{D}_{n-m,j}^- - \hat{D}_{n-m,j}^+) - \sum_{i \in \cI_{n-m}^c} D_i^+ = \Delta_{n-m}
        \quad \text{and} \quad
        \sum_{j=1}^{r-m} \hat{D}_{n-m, j}^- = \Xi^-_{n-m}.
    \end{equation*}
    Therefore,
    \begin{align*}
        \tilde{\gamma}^{n, m}_r (\vk_1, \ldots, \vk_m)
        &= \E \left[
            \frac{1}{p^m} \prod_{i=1}^m \frac{(r - i + 1) \mu}{\sum_{j=i}^m k_j^- + \Xi_{n-m}^-} \one_{A_n}
            \, \middle \vert \,
            R_{n-m} = r-m
        \right],
    \end{align*}
    where
    \begin{equation*}
        A_n(\vk_1, \ldots, \vk_m) = \left\{ \Delta_{n-m} =  \sum_{i=1}^m (k_i^+ - k_i^-) \right\}.
    \end{equation*}
    Hence,
    \begin{align*}
        \E \left[ 
            u\left( 
                \hat{\vD}_{n, 1}, \ldots, \hat{\vD}_{n, m}
             \right)
            \one\{R_n \geq m, \Delta_n = 0\}
         \right]
        =\E \left[ 
            u\left( \vZ_1, \ldots, \vZ_m \right)
            \tilde{\phi}^n_m(\vZ_1, \ldots, \vZ_m)
         \right],
    \end{align*}
    where
    \begin{align*}
        \tilde{\phi}^n_m(\vk_1, \ldots, \vk_m)
        &= \sum_{r=m}^n \binom{n}{r} p^r (1-p)^{n-r} 
        \E \left[
            \frac{1}{p^m} \prod_{i=1}^m \frac{(r - i + 1) \mu}{\sum_{j=i}^m k_j^- + \Xi_{n-m}^-} \one_{A_n}
            \, \middle \vert \,
            R_{n-m} = r-m
        \right] \\
        &= \sum_{l=1}^{n-m} \binom{n}{l+m} p^{l+m} (1-p)^{n-m-l} 
        \E \left[
            \frac{1}{p^m} \prod_{i=1}^m \frac{(l + m - i + 1) \mu}{\sum_{j=i}^m k_j^- + \Xi_{n-m}^-} \one_{A_n}
            \, \middle \vert \,
            R_{n-m} = l
        \right].
    \end{align*}
    We wish to view the sum as an expectation over $R_{n-m}$. In order to do this, we rewrite the expression so that we are taking a sum over the probabilities of a $\text{Binomial}(n-m, p)$ distribution. We can calculate
    \begin{equation*}
        \frac{\binom{n}{l+m} p^{l+m} (1-p)^{n-m-l}}{\binom{n-m}{l} p^l (1-p)^{n-m-l}}
        = p^m \prod_{i=1}^m \frac{(n-i+1)}{(l+m-i+1)}.
    \end{equation*}
    Therefore,
    \begin{align*}
        \tilde{\phi}^n_m(\vk_1, \ldots, \vk_m)
        &= \sum_{l=1}^{n-m} \binom{n-m}{l} p^l (1-p)^{n-m-l}
        \E \left[
            \prod_{i=1}^m \frac{(n - i + 1) \mu}{\sum_{j=i}^m k_j^- + \Xi_{n-m}^-} \one_{A_n}
            \, \middle \vert \,
            R_{n-m} = l
        \right] \\
        &= \E\left[ 
            \E \left[
                \prod_{i=1}^m \frac{(n - i + 1) \mu}{\sum_{j=i}^m k_j^- + \Xi_{n-m}^-} \one_{A_n}
                \, \middle \vert \,
                R_{n-m}
            \right]
         \right] \\
         &= \E \left[
            \prod_{i=1}^m \frac{(n - i + 1) \mu}{\sum_{j=i}^m k_j^- + \Xi_{n-m}^-} \one_{A_n}
        \right].
    \end{align*}
    Finally, dividing by $\P(R_n \geq m, \Delta_n = 0)$ yields the desired form of $\phi^n_m$.
\end{proof}

\subsection{Asymptotic lower bound on the measure change}

The following result, which is an analogue of \cite[Lemma 6.7]{conchon--kerjanStableGraphMetric2021}, describes the asymptotic behaviour of the measure change when $m = \Theta(n^{2/3})$.
\begin{lemma}
    \label{prop:measure-change-approx}
    Define
    \begin{equation*}
        s^{\pm}(i) = \textstyle{\sum_{j=1}^i (k_i^{\pm} - \lambda_{\pm})}.
    \end{equation*}
    Fix $\epsilon \in (0, 1/6)$ and suppose that $\vk_1, \ldots, \vk_m$ are such that
    \begin{equation}
        \label{eq:s-condition}
        \max_{i=1, \ldots, m} \abs{s^{\pm}(i)} \leq m^{\frac{1}{2} + \epsilon}.
    \end{equation}
    Then in the regime $m = \Theta(n^{2/3})$,
    \begin{equation*}
        \phi^n_m(\vk_1, \ldots, \vk_m)
        \geq \exp\left( \frac{1}{\mu n} \sum_{i=0}^m (s^-(i) - s^-(m)) - \frac{\sigma_-}{6 \mu^2} \frac{m^3}{n^2} \right) + \littleo(1),
    \end{equation*}
    where the $\littleo(1)$ term is independent of $\vk_1, \ldots, \vk_m$ satisfying our assumptions.
\end{lemma}
The $1/6$ upper bound on $\epsilon$ is used to show that certain terms that arise in the proof decay to 0. The exact value of $1/6$ is unimportant; rather, $\epsilon$ should be thought of as a positive constant we can make arbitrarily small to make the proof work. Let us explain the condition in \cref{eq:s-condition}. In \cref{thm:measure-change}, we evaluate $\phi^n_m$ as 
\begin{equation*}
    \phi^n_m(\vZ_1, \ldots, \vZ_m).
\end{equation*}
Thus the condition in \cref{eq:s-condition} corresponds to the event
\begin{equation*}
    \max_{i=1, \ldots, m } \abs*{
        \sum_{j=1}^i (Z^{\pm}_j - \lambda_{\pm}) 
    } \leq m^{1/2 + \epsilon}.
\end{equation*}
This says that the centered random walks corresponding to $Z^+_i$ and $Z^-_i$ do not deviate by more than $m^{1/2 + \epsilon}$ in the first $m$ steps. This event will occur with high probability, and so \cref{eq:s-condition} is not a restrictive condition to take.

The fact that we only prove a lower bound may seem strange at first. The idea is that since we are dealing with a measure change, as long as the lower bound will have expectation 1 in the limit, this shows that we have not lost a significant amount of probability mass. The following lemma, adapted from \cite[Lemma 4.8]{conchon--kerjanStableGraphMetric2021}, makes this formal.
\begin{lemma}
    \label{lem:sandwiching-lemma}
    Let $(X_n, Y_n, Z_n)_{n \geq 1}$ be a sequence of $[0, \infty) \times [0, \infty) \times S$-valued random variables where $S$ is a metric space. Suppose there exists a $[0, \infty) \times S$-valued random variable $(Y, Z)$ such that the following holds:
    \begin{enumerate}
        \item $(Y_n, Z_n) \todist (Y, Z)$ as $n \to \infty$.
        \item $X_n \geq Y_n$ almost surely for all $n$.
        \item $\E[X_n] = 1$ for all $n$ and $\E[Y] = 1$.
    \end{enumerate}
    Then $(X_n, Z_n) \todist (Y, Z)$ also. Moreover $(X_n)_{n \geq 1}$ is a sequence of uniformly integrable random variables.
\end{lemma}
\begin{proof}
    We first show $X_n - Y_n \to 0$ in $L^1$ as $n \to \infty$. Since $X_n \geq Y_n$,
    \begin{equation*}
        \limsup_{n \to \infty} \E \abs{X_n - Y_n}
        = \limsup_{n \to \infty} \E[X_n - Y_n]
        = 1 - \liminf_{n \to \infty} \E[Y_n].
    \end{equation*}
    Thus it suffices to show $\liminf_n \E[Y_n] \geq 1$. This follows since
    \begin{equation*}
        \liminf_n \E[Y_n] =
        \liminf_n \E[\abs{Y_n}] \geq
        \E[\abs{Y}] =
        \E[Y] = 1,
    \end{equation*}
    where the first and second equalities follow from the non-negativity of $Y_n$ and $Y$, and the inequality follows by the Portmanteau theorem.

    In particular $X_n - Y_n \todist 0$. Since this limit is a constant, it follows by Slutsky's theorem that
    \begin{equation*}
        \vectwo{X_n}{Z_n} = \vectwo{Y_n}{Z_n} + \vectwo{X_n - Y_n}{0} \todist \vectwo{Y}{Z}.
    \end{equation*}

    We now prove the uniform integrability. By Skorokhod's representation theorem we may suppose that $X_n \to Y$ almost surely. Then $\E[X_n] = \E[Y] = 1$ for all $n$. Therefore, $X_n \to Y$ in $L^1$ by Scheffé's lemma, which entails the required uniform integrability.
\end{proof}

\subsubsection{Exponential tilting}

Note that
\begin{equation*}
    \E[Z^- - Z^+] = \frac{1}{\mu} \E[D^-D^+ - (D^-)^2].
\end{equation*}
This quantity is, in general, non-zero, even if $\E[D^- - D^+] = 0$. The deviation of a sum of the $Z^{\pm}_i$ around its mean is controlled by the assumption in \cref{eq:s-condition}. If $\vk_1, \ldots, \vk_n$ satisfy \cref{eq:s-condition} and $m = \Theta(n^{2/3})$ then
\begin{equation*}
    \sum_{i=1}^m (k_i^- - k_i^+) = s^-(m) - s^+(m) + (\lambda_+ - \lambda_-) m = \Theta(n^{2/3}).
\end{equation*}

In contrast, $\Delta_{n-m}$ is centered, so
\begin{equation*}
    \left\{ \Delta_{n-m} = \textstyle \sum_{i=1}^m (k_i^+ - k_i^-) \right\}  
\end{equation*}
is looking at the event that $\Delta_{n-m}$ takes a value at distance $n^{2/3}$ away from its mean. As remarked in \cref{sec:llt}, the local limit theorem provides no information at distances $\omega(n^{1/2})$ from the mean since the error term will dominate.

In order to deal with this moderate deviation event, we will introduce a sequence of exponentially tilted measures, whose effect will be to shift the mean of $\Delta_{n-m}$ in such a way that, under the new measure, the event concerns only a typical deviation. The next result defines this tilt and then gives asymptotic expansions for cumulant generating function of $D^-$, the mean of $D^-$ and the mean of $D^+$ under this tilting. 
\begin{lemma}
    \label{lem:asym-expansions}
    Define an measure $\P_{\theta}$, for $\theta \geq 0$, by its Radon--Nikodym derivative
    \begin{equation*}
        \diff{\P_{\theta}}{\P} = \exp\left( - \theta D^- - \alpha(\theta) \right)
        \quad \text{where} \quad
        \alpha(\theta) = \log \E \left[ e^{-\theta D^-} \right].
    \end{equation*}
    Then as $\theta \downarrow 0$ we have
    \begin{align*}
        \alpha(\theta) &= -\mu \theta + \tfrac{1}{2}\var(D^-) \theta^2 - \tfrac{1}{6} \E \left[ (D^- - \mu)^3 \right] \theta^3 + \littleo(\theta^3), \\
        \E_{\theta}[D^-] &= \mu - \var(D^-) \theta + \bigo(\theta^3), \\
        \text{and} \quad \E_{\theta}[D^+] &= \mu - \cov(D^-, D^+) \theta + \bigo(\theta^3).
    \end{align*}
\end{lemma}
\begin{proof}
    Since $\E\left[\abs{D^-}^3\right] < \infty$ and $D^-$ is non-negative, by the dominated convergence theorem
    \begin{equation}
        \E \left[ (D^-)^3 \exp(-\theta D^-) \right] = \E \left[ (D^-)^3 \right] + \littleo(1)
        \label{eq:mgf-start}
    \end{equation}
    as $\theta \downarrow 0$. Integrating \cref{eq:mgf-start} with respect to $\theta$ and applying Fubini's theorem to exchange the order of the expectation and integral gives
    \begin{equation*}
        \E \left[ \int_0^{\theta} (D^-)^3 e^{-\theta' D^-} \dif \theta' \right]
        = \E \left[ \int_0^{\theta} \left\{ (D^-)^3 + \littleo(1) \right\} \dif \theta' \right]
        = \E \left[ (D^-)^3 \right] \theta + \littleo(\theta).
    \end{equation*}
    Evaluating the integral with respect to $\theta'$ on the left hand side and rearranging gives that
    \begin{equation*}
        \E \left[ (D^-)^2 e^{-\theta D^-} \right]
        = \E \left[ (D^-)^2 \right] - \E \left[ (D^-)^3 \right] \theta + \littleo(\theta).
    \end{equation*}
    Repeating this method yields
    \begin{align}
        \E \left[ D^- e^{-\theta D^-} \right]
        &= \mu - \E \left[ (D^-)^2 \right] \theta + \tfrac{1}{2} \E \left[ (D^-)^3 \right] \theta^2 + \littleo(\theta^2), \label{eq:asymin} \\
        \text{and} \quad \E \left[ e^{-\theta D^-} \right]
        &= 1 - \mu \theta + \tfrac{1}{2} \E \left[ (D^-)^2 \right] \theta^2 - \tfrac{1}{6} \E \left[ (D^-)^3 \right] \theta^3 + \littleo(\theta^3).
        \label{eq:asym00}
    \end{align}
    Similarly integrating the equation
    \begin{equation*}
        \E \left[ (D^-)^2 D^+ \exp(-\theta D^-) \right] = \E \left[ (D^-)^2 D^+ \right] + \littleo(1)
    \end{equation*}
    twice gives
    \begin{equation}
        \E \left[ D^+ e^{-\theta D^-} \right]
        = \mu \theta - \E \left[ D^- D^+ \right] \theta + \tfrac{1}{2} \E \left[ (D^-)^2 D^+ \right] \theta^2 + \littleo(\theta^2).
        \label{eq:asymout}
    \end{equation}
    \cref{eq:asym00} gives the small-$\theta$ expansion of the normalising constant of the measure change. Combining this with \cref{eq:asymin} and \cref{eq:asymout} yields the expansions for $\E_{\theta}[D^-]$ and $\E_{\theta}[D^+]$ respectively. Taking the logarithm of \cref{eq:asym00} gives the expansion of the cumulant generating function $\alpha(\theta)$.
\end{proof}

To achieve the recentering of $\Delta_{n-m}$ we desire, let us define a sequence of tilted measures $\P_n$ defined by their Radon--Nikodym derivative
\begin{equation}
    \diff{\P_n}{\P} = \exp \left( - \theta_n \Xi^-_{n-m} - (n - m) \alpha(\theta_n) \right),
\end{equation}
where $\theta_n = \frac{m}{\mu n}$. This factorises and so $\vD_1, \ldots, \vD_n$ remain i.i.d.\ under this tilting, each having the law of $\vD$ under $\P_{\theta_n}$. Applying \cref{lem:asym-expansions}, we can compute that
\begin{align*}
    \E_n[\Delta_{n-m}] 
    &= m(\lambda_+ - \lambda_-) + \bigo(n^{1/3}).
\end{align*}
Hence,
\begin{align*}
    \textstyle \sum_{i=1}^m (k_i^+ - k_i^-) - \E_n[\Delta_{n-m}] 
    &= s^-(m) - s^+(m) + \Big[ m(\lambda_+ - \lambda_-) - \E_n[\Delta_{n-m}] \Big] \\
    &= \bigo(n^{1/3 + \epsilon}),
\end{align*}
which is within the $\bigo(n^{1/2})$ range from the mean required for a typical deviation. This justifies our choice of $\theta_n = \frac{m}{\mu n}$.

It will turn out that the same exponential tilting is approximately achieved by the Radon-Nikodym derivative $\phi^n_m(\vk_1, \ldots, \vk_m)$, and so this perspective will play a key role in the proof of \cref{prop:measure-change-approx}.

\subsubsection{Local limit results}

We wish to determine the local limit behaviour of $\Delta_n$ under the untilted measure and $\Delta_{n-m}$ under the tilted measures. In the latter case, we wish to show the behaviour remains the same even when conditioning on $\Xi_{n-m}^-$ having fluctuations of order $\bigo(n^{1/2 + \epsilon})$ about its tilted mean. The way we show this is to first show a bivariate local limit theorem.

$(D^- - D^+, D^-)$ is $\Z^2$ valued and thus certainly lattice valued. Further, in the degenerate case where $D^- = D^+$ almost surely, the total in-degree and total out-degree will be equal almost surely and thus the conditioned and non-conditioned case are the same. So the proof of \cref{thm:measure-change} in that case is the same as that of \cite[Proposition 4.3]{conchon--kerjanStableGraphMetric2021}. Hence WLOG assume $(D^- - D^+, D^-)$ is non-degenerate. Let $\lattice$ be the main lattice of $(D^- - D^+, D^-)$. Then by \cref{lem:zd-triangular} there exist $p, q, r \in \Z_{\geq 0}$ such that $\lattice$ is generated by the columns of
\begin{equation*}
    \begin{pmatrix}
        p & 0 \\
        r & q
    \end{pmatrix}
\end{equation*}
We have assumed that $D^- - D^+$ has main lattice $\Z$ and therefore $p = 1$. Conditional on $D^- - D^+$ taking some value, $D^-$ will have main lattice $q \Z$. Let $\sigma^2$ be the variance of $D^- - D^+$ and $\Sigma$ be the covariance matrix of $(D^- - D^+, D^-)$.

We will show that $\P(R_n < m)$ decays exponentially and so the asymptotic behaviour of $\P(R_n \geq m, \Delta_n = 0)$ is dictated by the $\Delta_n = 0$ event. This can be handled by the standard local limit theorem.
\begin{lemma}
    \label{lem:normal-llt}
    As $n \to \infty$
    \begin{equation*}
        \P(R_n \geq m, \Delta_n = 0) = \frac{1}{\sqrt{2 \pi \sigma^2 n}} \left( 1 + \littleo(1) \right).
    \end{equation*}
\end{lemma}
\begin{proof}
    $R_n \sim \text{Binomial}(n, p)$ for $p > 0$ and, for sufficiently large $n$, $m \leq \frac{1}{2} pn$. So by Hoeffding's inequality,
    \begin{equation*}
        \P(\Delta_n = 0) - \P(R_n \geq m, \Delta_n = 0) \leq \P(R_n < m) \leq \P(\abs{R_n - np} < \tfrac{1}{2}pn) \leq e^{-cn}
    \end{equation*}
    for some $c > 0$.  The random variable $D^- - D^+$ is assumed to have finite variance $\sigma$ and main lattice $\Z$. Moreover it is centered and $0$ is in the main lattice $\Z$. Thus,
    \begin{equation*}
        \P(R_n \geq m, \Delta_n = 0) = \P(\Delta_n = 0) + \littleo(n^{-1/2}) = \frac{1}{\sqrt{2 \pi \sigma^2 n}}(1 + \littleo(1)),
    \end{equation*}
    where the second equality is by \cref{thm:normal-multi-llt}.
\end{proof}

Next we show the local limit theorem holds for $(\Delta_{n-m}, \Xi^-_{n-m})$ under the tilting.
\begin{lemma}
    \label{lem:bivar-llt}
    Let $\vc_n \in \Z^2$ be such that $\vc_n + \Lambda$ contains the support of $(\Delta_{n-m}, \Xi^-_{n-m})$. Then uniformly for $(x, y) \in \vc_n + \Lambda$,
    \begin{align*}
        &\P_n\left(
            \Delta_{n-m} = \E \big[ \Delta_{n-m} \big] + x, \ 
            \Xi^-_{n-m} = \E \big[ \Xi^-_{n-m} \big] + y
        \right)  \nonumber \\
        &\hspace{7em} = \frac{q}{2\pi \det(\Sigma)^{1/2} \: n} \exp\left( 
            \frac{-1}{2n}
            \begin{pmatrix}
                x & y
            \end{pmatrix}
            \Sigma
            \begin{pmatrix}
                x \\ y
            \end{pmatrix}
         \right)
         + \littleo( n^{-1} )
    \end{align*}
    as $n \to \infty$.
\end{lemma}
\begin{proof}
    Let $\vX_{n1}, \ldots, \vX_{nn}$ have the same distribution as 
    \begin{equation*}
        \vectwo{D^-_1 - D^+_1}{D^-_1}, \ldots, \vectwo{D^-_n - D^+_n}{D^-_n}
    \end{equation*}
    under the tilted measure $\P_n$. Then since $\theta_n = \littleo(1)$, it is simple to show that $\vX_{n1}$ tends weakly in law to $\vX = (D^- - D^+, D^-)$ under the non-tilted measure. The measure change does not change the support of the random variables and thus all $\vX_{n1}$ and $\vX$ have the same main lattice $\lattice$. Finally, we check the uniform integrability condition. Since $\theta_n = \littleo(1)$, we have $M = - \inf_n \alpha(\theta_n) < \infty$. Then
    \begin{align*}
        \sup_n \E[\norm{\vX_{n1}}^2 \one \{ \norm{\vX_{n1}}^2 \geq L \} ]
        &= \sup_n \E[e^{-\theta_n D^- - \alpha(\theta_n)} \norm{\vX}^2 \one\{\norm{\vX}^2 \geq L \} ] \\
        &\leq e^M \E[\norm{\vX}^2 \one\{\norm{\vX}^2 \geq L \} ] \\
        & \to 0
    \end{align*}
    as $L \to \infty$, since $\vX$ is assumed to have finite second moment. Thus the desired result follows from \cref{thm:multi-triangular-llt}. There is a slight change in that we have $n - m$ terms in the summations for $\Delta_{n-m}$ and $\Xi^-_{n-m}$ rather than $n$ terms, but since $m = \Theta(n^{2/3})$ this does not matter asymptotically.
\end{proof}

Now we show the $\P(\Delta_{n-m} = \sum_{i=1}^m (k_i^+ - k_i^-))$ have the same asymptotic behaviour as $\P(\Delta_n = 0)$ even when we condition on $\Xi_{n-m}^-$ not `varying too much' about its tilted mean. We only prove a lower bound, but this is sufficient for proving \cref{prop:measure-change-approx}.
\begin{lemma}
    \label{lem:mod-dev-local}
    Under the assumptions of \cref{prop:measure-change-approx},
    \begin{equation*}
        \mathbb P_n \left(
            \Delta_{n-m} = \sum_{i=1}^m (k_i^+ - k_i^-), \ 
            \abs{\Xi^-_{n-m} - \E_n[\Xi^-_{n-m}]} \leq n^{\frac{1}{2} + \epsilon}
        \right)
        \geq \frac{1}{\sqrt{2 \pi \sigma^2 n}} (1 + \littleo(1)).
    \end{equation*}
\end{lemma}
\begin{proof}
    For convenience let
    \begin{equation*}
        P_n = \mathbb P_n \left(
            \Delta_{n-m} = \sum_{i=1}^m (k_i^+ - k_i^-), \ 
            \abs{\Xi^-_{n-m} - \E_n[\Xi^-_{n-m}]} \leq n^{\frac{1}{2} + \epsilon}
        \right).
    \end{equation*}
    Define
    \begin{equation*}
        a_n = \sum_{i=1}^m (k_i^+ - k_i^-) - \E_n[\Delta_{n-m}].
    \end{equation*}
    Also let
    \begin{equation*}
        L_n = \Big\{
            y : \bigg( \textstyle\sum_{i=1}^m (k_i^+ - k_i^-), y \bigg) \in \vc_n + \lattice
            \Big\}.
    \end{equation*}
    $L_n$ has a simpler representation. Fix any $y_0 \in L_n$. Then if $\lattice$ is generated by the columns of
    \begin{equation*}
        \begin{pmatrix}
            1 & 0 \\
            r & q
        \end{pmatrix}
    \end{equation*}
    we must have $L_n = y_0 + q\Z$. Fix an arbitrary $M > 0$. Then
    \begin{align*}
        P_n &= \sum_{\substack{y \in L_n \\ \abs{y} \leq n^{1/2 + \epsilon}}} \mathbb P_n \left( \Delta_{n-m} = \E_n[\Delta_{n-m}] + a_n, \ \Xi^-_{n-m} = \E_n[\Xi^-_{n-m}] + y \right) \\
        &\geq \sum_{\substack{y \in L_n \\ \abs{y} \leq M n^{1/2}}} \mathbb P_n \left( \Delta_{n-m} = \E_n[\Delta_{n-m}] + a_n, \ \Xi^-_{n-m} = \E_n[\Xi^-_{n-m}] + y \right)
    \end{align*}
    for all $n$ sufficiently large. By \cref{lem:bivar-llt}, using that the error is uniform, we have that
    \begin{equation*}
        P_n \geq \sum_{\substack{y \in L_n \\ \abs{y} \leq M n^{1/2}}} 
         \frac{q}{2\pi \det(\Sigma)^{1/2} \: n} \exp\left( 
            \frac{-1}{2n} \vectwo{a_n}{y} \cdot \Sigma^{-1} \vectwo{a_n}{y}
         \right)
         + \littleo( n^{-1/2} )
    \end{equation*}

    We wish to factorise the summand. To this end, we make a change of variables. There exists $c \in \R$ such that
    \begin{equation*}
        \cov(D^- - c(D^- - D^+), D^- - D^+) = 0.
    \end{equation*}
    Let $\tau^2$ be the variance of $D^- - c(D^- - D^+)$. Then
    \begin{align*}
         &\frac{q}{2\pi \det(\Sigma)^{1/2} \: n} \exp\left( 
            \frac{1}{2n} \vectwo{a_n}{y} \cdot \Sigma^{-1} \vectwo{a_n}{y}
         \right) \nonumber \\
         & \hspace{5em} =
         \frac{1}{\sqrt{2 \pi \sigma^2 n}} \exp \left( - \frac{1}{2 \sigma^2} \frac{a_n^2}{n} \right)
         \frac{q}{\sqrt{2 \pi \tau^2 n}} \exp \left( - \frac{1}{2 \tau^2} \frac{(y - ca_n)^2}{n} \right).
    \end{align*}
    We now examine the asymptotic behaviour of $a_n$. By \cref{lem:asym-expansions},
    \begin{align*}
        \E_n[\Delta_{n-m}]
        &= (n - m) \E_{\theta_n}[D^- - D^+] \\ 
        &= -(\lambda_- - \lambda_+)m + \bigo(n^{1/3}).
    \end{align*}
    Therefore 
    \begin{equation*}
        a_n = s_+(m) - s_-(m) + \bigo(n^{1/3}) = \bigo(n^{1/3 + \epsilon}),
    \end{equation*}
    by the assumption in \cref{eq:s-condition}. Thus
    \begin{equation*}
        P_n \geq
        \frac{1}{\sqrt{2 \pi \sigma^2 n}}(1 + \littleo(1))
        \sum_{\substack{y \in L_n \\ \abs{y} \leq M n^{1/2}}}
        \frac{q}{\sqrt{2 \pi \tau^2 n}} \exp \left( - \frac{1}{2 \tau^2} \frac{(y - ca_n)^2}{n} \right)
        + \littleo(n^{-1/2})
    \end{equation*}
    Note that
    \begin{equation*}
        \sum_{\substack{y \in L_n \\ \abs{y} \leq M n^{1/2}}}
        \frac{q}{\sqrt{2 \pi \tau^2 n}} \exp \left( - \frac{1}{2 \tau^2} \frac{(y - ca_n)^2}{n} \right)
        = \sum_{\substack{y \in L_n \\ \abs{y} \leq M n^{1/2}}}
        \frac{q}{\sqrt{n}}\ g\left( \frac{y - ca_n}{\sqrt{n}} \right)
    \end{equation*}
    where
    \begin{equation*}
        g(z) = \frac{1}{\sqrt{2 \pi \tau^2}} \exp\left( \frac{-z^2}{2 \tau^2} \right).
    \end{equation*}
    Since $a_n = \bigo(n^{1/3 + \epsilon})$, for $n$ sufficiently large
    \begin{align}
        \sum_{\substack{y \in L_n \\ \abs{y} \leq M n^{1/2}}}
        \frac{q}{\sqrt{2 \pi \tau^2 n}} \exp \left( - \frac{1}{2 \tau^2} \frac{(y - ca_n)^2}{n} \right)
        &\geq \sum_{\substack{z \in L_n - ca_n\\ \abs{z} \leq \frac{1}{2} M n^{1/2}}} 
        \frac{q}{\sqrt{n}}\ g \left( \frac{z}{\sqrt{n}} \right) \\
        &= \sum_{\substack{z \in \tilde{L}_n \\ \abs{z} \leq \frac{1}{2} M }}
        \frac{q}{\sqrt{n}}\ g(z) \label{eq:riemann-sum}
    \end{align}
    where
    \begin{equation*}
        \tilde{L}_n = \frac{L_n - ca_n}{\sqrt{n}}.
    \end{equation*}
    Then $\tilde{L}_n \cap [-\frac{1}{2}M, \frac{1}{2}M]$ is a partition of $[-\frac{1}{2}M, \frac{1}{2}M]$ where adjacent points are distance $q/\sqrt{n}$ apart from each other. Thus \cref{eq:riemann-sum} is a Riemann sum approximation of an integral. Hence
    \begin{equation*}
        \sum_{\substack{y \in L_n \\ \abs{y} \leq M n^{1/2}}}
        \frac{q}{\sqrt{2 \pi \tau^2 n}} \exp \left( - \frac{1}{2 \tau^2} \frac{(y - ca_n)^2}{n} \right)
        \geq (1 + \littleo(1)) \int_{-\frac{1}{2} M}^{\frac{1}{2}M} g(z) \dif z.
    \end{equation*}
    Thus
    \begin{equation*}
        P_n \geq \frac{1}{\sqrt{2 \pi \sigma^2 n}} (1 + \littleo(1)) \int_{-\frac{1}{2} M}^{\frac{1}{2}M} g(z) \dif z.
    \end{equation*}
    This holds for all $M > 0$, and $\int_{-\infty}^{\infty} g(z) \dif z = 1$. Therefore,
    \begin{equation*}
        P_n \geq \frac{1}{\sqrt{2 \pi \sigma^2 n}} \left( 1 + \littleo(1) \right),
    \end{equation*}
    as required.
\end{proof}

\subsubsection{Poof of the asymptotic lower bound}

We are now ready to prove \cref{prop:measure-change-approx}.
\begin{proof}[Proof of \cref{prop:measure-change-approx}]
    Firstly,
    \begin{equation*}
        \prod_{i=1}^m \frac{(n-i+1)\mu}{\sum_{k=i}^m k^-_i + \Xi^-_{n-m}} = \exp(X_n - Y_n),
    \end{equation*}
    where
    \begin{equation*}
        X_n = \sum_{i=1}^m \log\left( 1 - \frac{i-1}{n} \right)
        \quad \text{and} \quad
        Y_n = \sum_{i=1}^m \log\left( \frac{\sum_{k=i}^m k_i^- + \Xi^-_{n-m}}{\mu n} \right).
    \end{equation*}
    Note that
    \begin{equation*}
        \sum_{j=i}^m k^-_j = s^-(m) - s^-(i - 1) + (m - i + 1) \lambda_-,
    \end{equation*}
    and define
    \begin{equation*}
        \Omega^-_n = \Xi^-_{n-m} - (n-m)\mu + (\lambda_- + \mu)m.
    \end{equation*}
    Then $\Omega_n^-$ is almost the centering of $\Xi_{n-m}^-$ under $\P_n$. We have
    \begin{align*}
        Y_n 
        &= \sum_{i=1}^m \log \left( \frac{s^-(m) - s^-(i-1) + (m - i + 1) \lambda_- + \Omega^-_n + \mu n - \lambda_- m}{\mu n} \right) \\
        &= \sum_{i=1}^m \log \left( 1 + A_n^i + B_n + C_n^i \right)
    \end{align*}
    where
    \begin{align*}
        A_n^i = - \frac{1}{\mu n} \left[ s^-(i-1) - s^-(m) \right], \quad
        B_n = \frac{1}{\mu n} \Omega^-_n, \quad
        C_n^i = - \frac{\lambda_-}{\mu n} (i-1).
    \end{align*}
    The summation contributes order $m = O(n^{2/3})$. Thus we keep terms of order $\Omega(n^{-2/3})$ when expanding $\log(1 + A_n^i + B_n + C_n^i)$. Write
    \begin{equation*}
        \omegaEvent_n = \left\{ \abs{\Omega^-_n} \leq 2n^{\frac{1}{2} + \epsilon} \right\}.
    \end{equation*}
    On the event $\omegaEvent_n$, we can check that the $A_n^i, B_n, C_n^i$ and $(C_n^i)^2$ terms are the only ones in the expansion which have order $\Omega(n^{-2/3})$. Moreover,
    \begin{equation*}
        \sum_{i=1}^m C_n^i = - \frac{\lambda_-}{2 \mu} \frac{m^2}{n} + \littleo(1) \quad \text{and} \quad
        \sum_{i=1}^m (C_n^i)^2 = \frac{\lambda_-^2}{3 \mu^2} \frac{m^3}{n^2} + \littleo(1).
    \end{equation*}
    Therefore,
    \begin{align*}
        Y_n
        &= \sum_{i=1}^m (A_n^i + B_n + C_n^i - \tfrac{1}{2} (C_n^i)^2) + \littleo(1) \\
        &= - \frac{1}{\mu n} \sum_{i=0}^m \left( s^-(i) - s^-(m) \right)
        + \frac{m}{\mu n} \Omega_n^-
        - \frac{\lambda_-}{2\mu} \frac{m^2}{n} - \frac{\lambda_-^2}{6 \mu^2} \frac{m^3}{n^2} + \littleo(1),
    \end{align*}
    where we use that $\sum_{i=1}^m \left( s^-(i-1) - s^-(m) \right) = \sum_{i=0}^m \left( s^-(i) - s^-(m) \right)$.

    Similarly we can expand $X_n$ as
    \begin{equation*}
        X_n = - \frac{m}{2 n} - \frac{m^3}{3 n^2} + \littleo(1).
    \end{equation*}

    Thus,
    \begin{align*}
        \prod_{i=1}^m \frac{(n-i+1)\mu}{\sum_{k=i}^m k^-_i + \Xi^-_{n-m}}
        &\geq \exp \Bigg( \frac{1}{\mu n} \sum_{i=1}^m (s^-(i) - s^-(m)) \nonumber \\
        &\hspace{4em} - \frac{m}{\mu n} \Omega^-_n + \frac{(\lambda_- - \mu)}{2 \mu} \frac{m^2}{n} + \frac{(\lambda_-^2 - \mu^2)}{6 \mu^2} \frac{m^3}{n^2} \Bigg) \one_{\omegaEvent_n}.
    \end{align*}
    In addition, using \cref{lem:asym-expansions}, the measure change can be expanded as
    \begin{equation*}
        \diff{\P_n}{\P} = \exp \left( 
            - \frac{m}{\mu n} \Omega_n^- + \frac{(\lambda_- - \mu)}{2\mu} \frac{m^2}{n}
            + \frac{(\lambda_-^2 - \mu^2)}{6 \mu^2} \frac{m^3}{n^2} + \frac{\sigma_-}{6 \mu^2} \frac{m^3}{n^2} + \littleo(1)
         \right).
    \end{equation*}
    Hence,
    \begin{align*}
        &\phi^n_m(\vk_1, \ldots, \vk_m) \\
        =& \frac{1}{\P(R_m \geq n, \Delta_n = 0)} \E \left[\prod_{i=1}^m \frac{(n-i+1)\mu}{\sum_{k=i}^m k^-_i + \Xi^-_{n-m}} \one_{A_n} \right] \\
        \geq& \frac{1}{\P(R_n \geq m, \Delta_n = 0)} \E_n \left[ \exp \left(
                \frac{1}{\mu n} \sum_{i=1}^m \left( s^-(i) - s^-(m) \right)
                - \frac{\sigma_-}{6 \mu^2} \frac{m^3}{n^2} + \littleo(1)
            \right) \one_{\omegaEvent_n \cap A_n} \right] \\
        \geq& \exp \left(
                \frac{1}{\mu n} \sum_{i=1}^m \left( s^-(i) - s^-(m) \right)
                - \frac{\sigma_-}{6 \mu^2} \frac{m^3}{n^2}
            \right) (1 + \littleo(1)) \frac{\P_n(\omegaEvent_n \cap A_n)}{\P(R_m \geq n, \Delta_n = 0)}.
    \end{align*}
    By \cref{lem:asym-expansions} we have that
    \begin{equation*}
        \Omega^-_n = \Xi^-_{n-m} - \E_n[\Xi^-_{n-m}] + \bigo(n^{1/3}).
    \end{equation*}
    In particular, for all sufficiently large $n$,
    \begin{equation*}
        \P_n(\omegaEvent_n \cap A_n) \geq
        \P_n\left(
            \abs{\Xi^-_{n-m} - \E[\Xi^-_{n-m}]} \leq n^{1/2 + \epsilon}, \Delta_{n-m} = \sum_{i=1}^m (k^+_i - k^-_i)
        \right).
    \end{equation*}
    Thus by \cref{lem:normal-llt,lem:mod-dev-local},
    \begin{equation*}
        \frac{\P_n(\omegaEvent_n \cap A_n)}{\P(R_n \geq m, \Delta_n = 0)} \geq 1 + \littleo(1)
    \end{equation*}
    as $n \to \infty$, which gives the desired final result.
\end{proof}

\subsection{Convergence of the measure change}

We are now ready to prove the main result of this section.

\begin{proof}[Proof of \cref{prop:measure-change-no-crit}]
    The existence of the measure change is covered by \cref{lem:exact-measure-change}. Define
    \begin{equation*}
        \Gamma(n, m) = \exp \left( 
            \frac{1}{\mu n} \sum_{i=0}^m \left( 
                V^-(i) - V^-(m)
             \right)
             - \frac{\sigma_-}{6 \mu^2} \frac{m^3}{n^2}
         \right).
    \end{equation*}
    Then by Donsker's invariance principle,
    \begin{equation*}
        \left( 
            n^{-1/3} V^-(\floor{tn^{2/3}}),
            n^{-1/3} V^+(\floor{tn^{2/3}})
         \right)_{t \geq 0} \todist
         \left( 
             \sigma_- W^-_t,
             \sigma_+ W^+_t
          \right)_{t \geq 0}
    \end{equation*}
    in $\D\left([0, \infty), \R^2\right)$, where $(W^-_t, W^+_t)_{t \geq 0}$ are a pair of correlated standard Brownian motions with correlation $\corr(Z^-_1, Z^+_1)$. We can write
    \begin{align*}
        \frac{1}{n} \sum_{i=0}^{\floor{T n^{2/3}}} V^-(i)
        &= n^{-2/3} \int_0^{\floor{T n^{2/3}} + 1} n^{-1/3} V^-(\floor{u}) \dif u \\
        &= \int_0^{n^{-2/3}(\floor{T n^{2/3} + 1})} n^{-1/3} V^-(\floor{s n^{2/3}}) \dif s.
    \end{align*}
    Thus, by the continuous mapping theorem,
    \begin{align*}
        \frac{1}{n} \sum_{i=0}^{\floor{T n^{2/3}}} \left(V^-(i) - V^-(m) \right)
        &\todist \int_0^T \left(W^-_s - W^-_T \right) \dif s
        = - \int_0^T s \dif W^-_s.
    \end{align*}
    Hence,
    \begin{align*}
        &\left( 
            \Gamma(n, \floor{T n^{2/3}}),
            \left(
                n^{-1/3} V^-(\floor{t n^{2/3}}),
                n^{-1/3} V^+(\floor{t n^{2/3}})
            \right)_{t \in [0, T]}
         \right) \\
         &\hspace{22em} \todist
         \left( 
             \Phi(T), (\sigma_- W^-_t, \sigma_+ W^+_t)_{t \in [0, T]}
          \right)
    \end{align*}
    in $\R \times \D([0, T], \R)$, as $n \to \infty$. Define the event
    \begin{equation*}
        E_m = \left\{ 
            \max_{i=1, \ldots, m} \abs{V^-(i)} \leq m^{1/2 + \epsilon}
            \quad \text{and} \quad
            \max_{i=1, \ldots, m} \abs{V^+(i)} \leq m^{1/2 + \epsilon}
         \right\}
    \end{equation*}
    for $\epsilon \in (0, 1/6)$. By \cref{prop:measure-change-approx}, it is the case that
    \begin{equation*}
        \Phi(n, m) \geq (\Gamma(n, m) + \littleo(1)) \one_{E_m}.
    \end{equation*}
    The processes $(V^{\pm}(n))_{n \geq 0}$ are discrete martingales. Therefore, by Doob's maximal inequality,
    \begin{equation*}
        \P\left(\max_{i=1, \ldots, m} \abs{V^{\pm}(i)} > m^{1/2 + \epsilon}\right)
        \leq \frac{\E[(V^{\pm}(m))^2]}{m^{1 + 2 \epsilon}} = \frac{\sigma_{\pm}^2}{m^{2 \epsilon}} \to 0
    \end{equation*}
    as $m \to \infty$. Thus $\P(E_m) \to 1$ as $m \to \infty$. Hence, we still have that
    \begin{align*}
        &\left( 
            (\Gamma(n, \floor{T n^{2/3}}) + \littleo(1))\one_{E_{\floor{T n^{2/3}}}} ,
            \left(
                n^{-1/3} V^-(\floor{t n^{2/3}}),
                n^{-1/3} V^+(\floor{t n^{2/3}})
            \right)_{t \in [0, T]}
         \right) \\
         & \hspace{22em} \todist
         \left( 
             \Phi(T), (\sigma_- W^-_t, \sigma_+ W^+_t)_{t \in [0, T]}
          \right).
    \end{align*}
    We have $\E[\Phi(T)] = 1$ by a standard stochastic calculus calculation. Therefore, by \cref{lem:sandwiching-lemma}, we get the desired result that
    \begin{align*}
        &\left( 
            \Phi(n, \floor{T n^{2/3}}) ,
            \left(n^{-1/3} V^-(\floor{t n^{2/3}}), n^{-1/3} V^+(\floor{t n^{2/3}}) \right)_{t \in [0, T]}
         \right) \\
        & \hspace{22em} \todist
         \left( 
             \Phi(T), (\sigma_- W^-_t, \sigma_+ W^+_t)_{t \in [0, T]}
          \right),
    \end{align*}
    and that $(\Phi(n, \floor{T n^{2/3}}))_{n \geq 1}$ is a uniformly integrable sequence.
\end{proof}
